# Supplementary material for: NormSAGE: Multi-Lingual Multi-Cultural Norm Discovery from Conversations On-the-Fly
Source: arXiv:2210.08604 source file (2024-01-13)
Supplement: Supplementary file 1 [file appendix.tex]

\section{Appendix}
In Table \ref{tab:templates}, we provide the full list of templates we used for prompting norm discovery. In Table \ref{fig:TurkUI}, we show an example annotation interface for norm comparisons.

\input{tables/table7.tex}

\begin{figure*}[t]
\frame{\includegraphics[scale=0.97]{figures/TurkUI.pdf}}
\caption{We first provide annotators with a reminder definition of what is a "\textbf{norm}". Then, we describe the metric of assessment for the norm in this HIT and make sure that they understand, with a confirmation of "\textit{Yes}". Finally, we ask the annotators to rank each set of norms, de-identified and randomized from the different norm discovery approaches, on a Likert Scale. The Mechanical Turk UI makes sure that the annotators have moved the scale values around before the HIT can be submitted successfully.}
\label{fig:TurkUI}
\end{figure*}
